# Supplementary material for: Evaluating Distributed Representations for Multi-Level Lexical Semantics: A Research Proposal
Source: arXiv:2406.00751 source file (2024-12-03)
Supplement: Supplementary file 1 [file Appendix.tex]

\appendix

\section{Appendix}
\label{sec:appendix}

\subsection{Optimal Thresholds for each layer}
\label{sec:threshold}
We list the optimal thresholds for each layer in terms of three settings of Llama2, i.e., base, repeat and prompt in Table~\ref{app_tab:thresholds}. They are searched according to the best performance in the development set of WiC dataset.

\begin{table}[h]
    \centering
    \begin{tabular}{cccc}
    \toprule
        Layer Index & base & repeat & prompt \\
        \midrule
         0&0.95&0.95&0.40\\
1&0.90&0.90&0.35\\
2&0.55&0.75&0.25\\
3&0.70&0.70&0.40\\
4&0.45&0.55&0.30\\
5&0.35&0.45&0.40\\
6&0.35&0.40&0.35\\
7&0.30&0.35&0.35\\
8&0.25&0.25&0.35\\
9&0.25&0.25&0.35\\
10&0.35&0.25&0.40\\
11&0.35&0.20&0.35\\
12&0.30&0.25&0.40\\
13&0.30&0.35&0.35\\
14&0.35&0.30&0.40\\
15&0.45&0.35&0.45\\
16&0.40&0.40&0.50\\
17&0.40&0.35&0.55\\
18&0.45&0.40&0.45\\
19&0.45&0.35&0.55\\
20&0.45&0.40&0.55\\
21&0.45&0.40&0.45\\
22&0.40&0.35&0.55\\
23&0.35&0.35&0.60\\
24&0.40&0.35&0.60\\
25&0.35&0.30&0.50\\
26&0.40&0.25&0.50\\
27&0.40&0.45&0.55\\
28&0.30&0.25&0.50\\
29&0.35&0.45&0.50\\
30&0.35&0.40&0.55\\
31&0.40&0.35&0.55\\
\bottomrule
    \end{tabular}
    \caption{Optimal thresholds for each layer.}
    \label{app_tab:thresholds}
\end{table}
